# Supplementary material for: BusReF: Infrared-Visible images registration and fusion focus on reconstructible area using one set of features
Source: arXiv:2401.00285 source file (2023-12-30)
Supplement: Supplementary file 1 [file X_suppl.tex]

\clearpage
\setcounter{page}{1}
\maketitlesupplementary

\section{Study of Fine Registration}
Ideally, in most multi-camera systems, a general affine transformation would be sufficient for registration. However, due to the different inside and outside camera parameters , as well as possible timing delays, the moving objects captured by the multi-camera may have some elastic deformation. Therefore we need to further refine the results by deformation field.
\begin{figure}
    \begin{center}
        \includegraphics[trim={0mm 0mm 0mm 0mm},clip,width=1\linewidth]{sec/pdfs/aug_example.pdf}
        \caption{Example of augmentation.}\label{augmentation}
    \end{center}
\end{figure}
\subsection{The Generation of Deformation Field}\label{df_generation}
Firstly we assume that the size of the image to be aligned is $[H,W]$. Initially, the 2D Gaussian kernel $G[i,j]$ with the size of $(2k+1)*(2k+1)$:
\begin{equation}\label{gaussion}
    G[x,y]=\frac 1 { 2\pi\sigma^2 }{\exp}\left[{-\frac {(x-k-1)^2+(y-k-1)^2}{2\sigma^2}}\right],
\end{equation}
where $\sigma$ here is empirically set to 32.
Randomly initialise the noise matrix $n_x, n_y$ of size $[H,W]$ and apply Gaussian filter on it:
    \begin{equation}
        [d_x,d_y] = [G(n_x),G(n_y)],
    \end{equation}
where $G()$ stands for Gaussian filtering of inputs, the offset matrices $d_x, d_y$ represent the pixel displacement of the moving image on $x, y$ axes respectively. Finally, we concatenate $d_x$ and $d_y$ to get the deformation field $\phi$:
\begin{equation}
    \phi = Concat(d_x,d_y)
\end{equation}
Figure ~\ref{augmentation} illustrates the affine transformations and deformation fields used in this paper.
\subsection{Elastic Deformation}
\begin{figure*}
    \begin{center}
        \includegraphics[trim={0mm 0mm 0mm 0mm},clip,width=0.9\linewidth]{sec/pdfs/studyelastic.pdf}
        \caption{Coarse and fine alignment results of BusReF at various levels of distortion.}
    \end{center}
\end{figure*}
% Please add the following required packages to your document preamble:
% \usepackage{graphicx}
% \usepackage[table,xcdraw]{xcolor}
% Beamer presentation requires \usepackage{colortbl} instead of \usepackage[table,xcdraw]{xcolor}
\begin{table}[]
\centering
\caption{NCC performance of BusReF on RoadScene dataset under different $k$ settings.}
\label{study_elastic}
\resizebox{\columnwidth}{!}{%
\fontsize{3}{4}\selectfont
\begin{tabular}{c|cccc}
\hline
{\color[HTML]{000000} Deformation Field} & {\color[HTML]{000000} \scalebox{0.6}{$k$}=30} & {\color[HTML]{000000} \scalebox{0.6}{$k$}=25} & {\color[HTML]{000000} \scalebox{0.6}{$k$}=20} & {\color[HTML]{000000} \scalebox{0.6}{$k$}=15} \\ \hline
W & 0.872 & 0.869 & 0.866 & 0.858 \\
W/O & 0.862 & 0.859 & 0.856 & 0.849 \\ \hline
\end{tabular}%
}
\end{table}
We visualised the registration of deformation field. In Equation ~\ref{gaussion}, the value of $k$ determines the magnitude of the numerical fluctuations in the offset matrix. Note that the larger of the $k$, the stronger the filtering effect and the smaller the fluctuation of the offset matrix value, which is reflected in the image with a smaller degree of elastic deformation. By visualizing and calculating quantitative metrics for different $k$, the adaptability of BusReF to different degrees of elastic deformation was surveyed in Table ~\ref{study_elastic}. From the visualisation results, when $k=30, 25$, our algorithm is still able to produce a suitable deformation field to fit the elastic deformation. When $k=20, 15$, the image is severely distorted and the deformation field cannot fully fit the image. However, such severe distortions are rare in real scene, and our affine transformation module also completes the alignment of the rigid transformation to some extent.
\section{Training Details}
% Please add the following required packages to your document preamble:
% \usepackage{graphicx}
\begin{table}[]
\centering
\caption{A brief description of the datasets used in the study.}
\label{datasets}
\resizebox{\columnwidth}{!}{%
\fontsize{3}{4}\selectfont
\begin{tabular}{c|cccc}
\hline
Source &  Modality & Size & Train or Test & Resize \\ \hline\hline
LLVIP & TIR-VI & 15488 & Train & 256\scalebox{0.6}{$\times$}256 \\
MSRS & TIR-VI & 1444 & Train & 256\scalebox{0.6}{$\times$}256 \\
RoadScene & TIR-VI & 221 & Test & 256\scalebox{0.6}{$\times$}256 \\
NIRScene & NIR-VI & 469 & Test & 256\scalebox{0.6}{$\times$}256 \\ \hline

\end{tabular}%z
}

\end{table}

Our training data comes from 15488 pairs of images from LLVIP~\cite{Jia_2021_ICCV} and 1444 pairs of images from MSRS~\cite{8206396,TANG202279}, which are two strictly aligned thermal infrared-visible image datasets. When training the reconstructor, we mix all images from both modalities, which represents the reconstructor is able to extract and reconstruct information from both modalities. 
% The reconstructor is judged to have converged when its average loss no longer decreases for three consecutive epochs, and the registration module is mounted for bus like training.

While training the registration modules we randomly sampled the corresponding image pairs from LLVIP and MSRS and performed artificial affine and elastic transformations on them. During testing phase, we chose 221 pairs of images from RoadScene~\cite{9151265} as the dataset for thermal infrared and 469 pairs of images from NIRScene~\cite{5995637} as the dataset for near infrared.
In Table~\ref{datasets} we give the datasets required for training. For training the bus we used a mixed dataset of LLVIP and MSRS totalling 33864 IR-Vis images. The bus was trained with 5 Epochs, the optimiser was Adam and the learning rate was 0.0001. After that we mounted on Affine Net and Deformable Net for registration training. For the affine transformations used include ±10 degrees of rotation, random displacement of 25 pixel points on the left, right, top and bottom, scaling from 0.9 to 1.1 magnification, and ±5 degrees of shear transformation. The registration modules was trained for 30 epochs, with the optimiser being Adam, with a learning rate of 0.0001 and learning rate decay in the last 10 epochs.
